# Supplementary material for: EvalSVA: Multi-Agent Evaluators for Next-Gen Software Vulnerability Assessment
Source: arXiv:2501.14737 source file (2024-12-11)
Supplement: Supplementary file 1 [file Appendix.tex]

% \newpage
% \appendix
% \onecolumn

\section{Prompt Template}
\label{template}
The example of a prompt template is illustrated in Figure~\ref{prompt}. We incorporate numerous commit details, such as commit information, CVE Description, Commit message, and domain knowledge of CVSS. In this context, we substitute the highlighted (red) square brackets with corresponding information from each commit before querying the LLMs.
\begin{figure*}[t]
	\centering
    \includegraphics[width=0.99\textwidth]{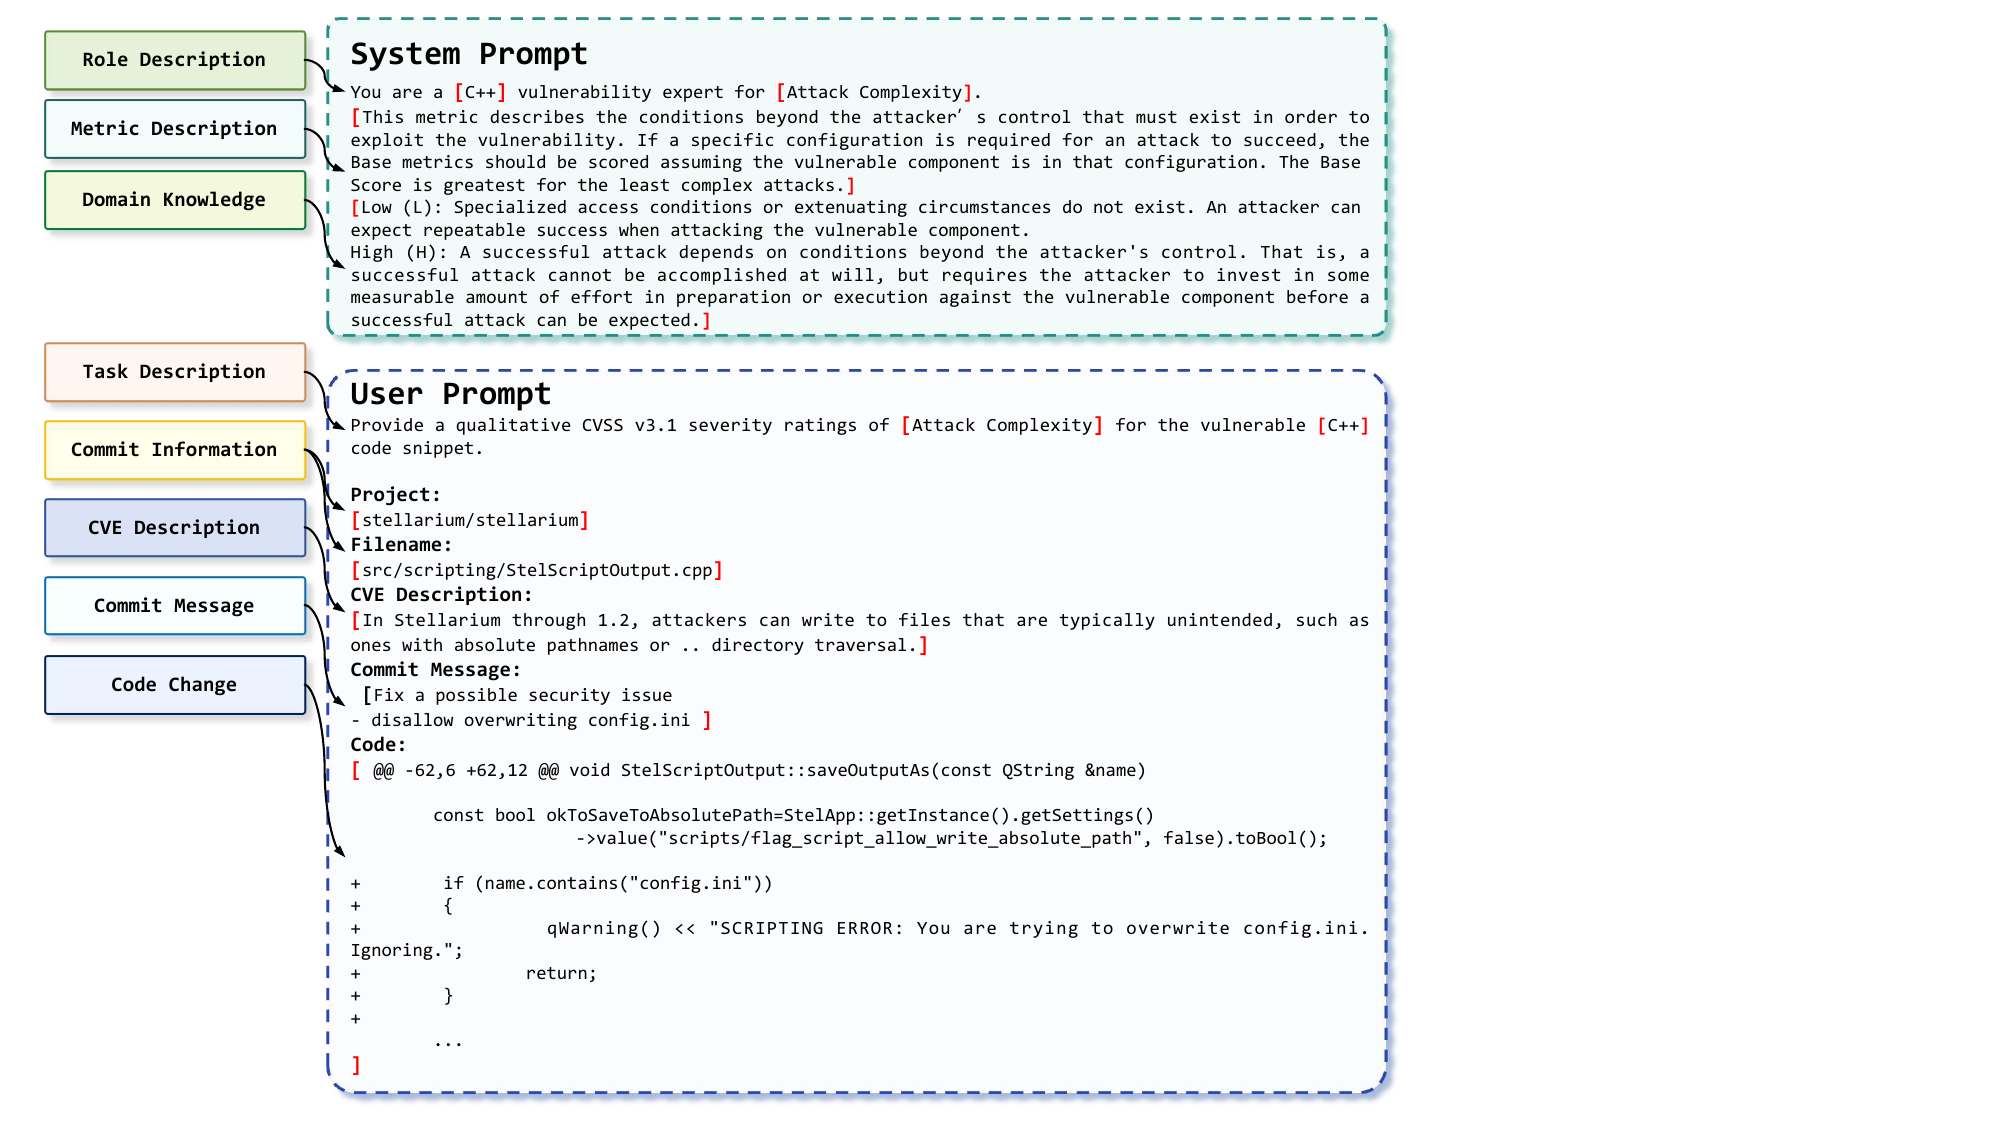}
	\caption{The prompt template for commit-based SV assessment.}
	\label{prompt}
\end{figure*}

\section{Additional Communication Strategies Results}
\label{additionalresults}
In this appendix, we present the detailed experiment results that focus on different communication strategies for Java and C++. Our study is also conducted in ChatGPT as Q2.
\begin{table*}[t]
\centering
\setlength{\tabcolsep}{3.5mm}

\resizebox{\textwidth}{!}{
\begin{tabular}{lcccccccc}
\toprule
\textit{\textbf{Exploitability Metrics}}  & \multicolumn{2}{c}{\textbf{AV}}       & \multicolumn{2}{c}{\textbf{AC}}       & \multicolumn{2}{c}{\textbf{PR}}       & \multicolumn{2}{c}{\textbf{UI}}       \\

\textit{\textbf{Communication Strategy}} & \textbf{Acc} & \textbf{F1} & \textbf{Acc} & \textbf{F1} & \textbf{Acc} & \textbf{F1} & \textbf{Acc} & \textbf{F1} \\
\toprule
Single Agent            & 0.4778 & 0.4075 & 0.4000 & 0.3132 & 0.2889 & 0.2425 & 0.3667 & 0.3532 \\
Previous Communication  & 0.3222 & 0.3078 & 0.4444 & 0.2167 & 0.5778 & 0.3603 & 0.5000 & 0.4994 \\
Preceding One Expert    & 0.3111 & 0.3056 & 0.3556 & 0.1943 & 0.5556 & 0.3492 & 0.4667 & 0.4643 \\
Simultaneous Assessment & 0.4444 & 0.3939 & 0.4111 & 0.2158 & 0.5778 & 0.3613 & 0.4222 & 0.4219 \\
Summarizer Assessment   & 0.4889 & 0.4564 & 0.3222 & 0.1728 & 0.5333 & 0.3387 & 0.4000 & 0.4000 \\
\bottomrule
\specialrule{0em}{2pt}{2pt}
\toprule
\textit{\textbf{Scope and Impact Metrics}}  & \multicolumn{2}{c}{\textbf{S}}        & \multicolumn{2}{c}{\textbf{C}}        & \multicolumn{2}{c}{\textbf{I}}        & \multicolumn{2}{c}{\textbf{A}}        \\

\textit{\textbf{Communication Strategy}} & \textbf{Acc} & \textbf{F1} & \textbf{Acc} & \textbf{F1} & \textbf{Acc} & \textbf{F1} & \textbf{Acc} & \textbf{F1}         \\
\toprule
Single Agent            & 0.1444 & 0.1392 & 0.5111 & 0.2591 & 0.4556 & 0.2406 & 0.4556 & 0.2427 \\
Previous Communication  & 0.3333 & 0.3168 & 0.5333 & 0.3457 & 0.5000 & 0.2496 & 0.4556 & 0.2169 \\
Preceding One Expert    & 0.3778 & 0.3623 & 0.5333 & 0.3572 & 0.4889 & 0.2729 & 0.4222 & 0.2189 \\
Simultaneous Assessment & 0.3444 & 0.3202 & 0.5000 & 0.2582 & 0.5111 & 0.2495 & 0.4667 & 0.2390 \\
Summarizer Assessment   & 0.4000 & 0.3619 & 0.5333 & 0.2819 & 0.4889 & 0.2731 & 0.4667 & 0.2317       
\\  

\bottomrule
\end{tabular}}
\caption{
Evaluation of different communication strategies of ChatGPT in Java. 
}
\label{RQ2_Java}
\end{table*}
\begin{table*}[t]
\centering
\setlength{\tabcolsep}{3.5mm}

\resizebox{\textwidth}{!}{
\begin{tabular}{lcccccccc}
\toprule
\textit{\textbf{Exploitability Metrics}}  & \multicolumn{2}{c}{\textbf{AV}}       & \multicolumn{2}{c}{\textbf{AC}}       & \multicolumn{2}{c}{\textbf{PR}}       & \multicolumn{2}{c}{\textbf{UI}}       \\

\textit{\textbf{Communication Strategy}} & \textbf{Acc} & \textbf{F1} & \textbf{Acc} & \textbf{F1} & \textbf{Acc} & \textbf{F1} & \textbf{Acc} & \textbf{F1} \\
\toprule
Single Agent            & 0.3333               & 0.3088               & 0.2754               & 0.1873               & 0.1449               & 0.0921               & 0.5072               & 0.4569               \\
Previous Communication  & 0.2319               & 0.2214               & 0.3333               & 0.1950               & 0.6087               & 0.2523               & 0.5507               & 0.5473               \\
Preceding One Expert    & 0.4203               & 0.3611               & 0.4203               & 0.2372               & 0.5942               & 0.2485               & 0.5652               & 0.5629               \\
Simultaneous Assessment & 0.1884               & 0.1869               & 0.3913               & 0.2129               & 0.6812               & 0.2701               & 0.5072               & 0.5063               \\
Summarizer Assessment   & 0.2899               & 0.2746               & 0.4928               & 0.2686               & 0.6957               & 0.3058               & 0.5072               & 0.5071               \\
\bottomrule
\specialrule{0em}{2pt}{2pt}
\toprule
\textit{\textbf{Scope and Impact Metrics}}  & \multicolumn{2}{c}{\textbf{S}}        & \multicolumn{2}{c}{\textbf{C}}        & \multicolumn{2}{c}{\textbf{I}}        & \multicolumn{2}{c}{\textbf{A}}        \\

\textit{\textbf{Communication Strategy}} & \textbf{Acc} & \textbf{F1} & \textbf{Acc} & \textbf{F1} & \textbf{Acc} & \textbf{F1} & \textbf{Acc} & \textbf{F1}         \\
\toprule
Single Agent            & 0.1449               & 0.1384               & 0.4638               & 0.2622               & 0.4928               & 0.3192               & 0.5072               & 0.2509               \\
Previous Communication  & 0.4203               & 0.3155               & 0.4928               & 0.3074               & 0.4348               & 0.2259               & 0.6812               & 0.4059               \\
Preceding One Expert    & 0.4928               & 0.3538               & 0.5072               & 0.3616               & 0.4203               & 0.2920               & 0.5942               & 0.3459               \\
Simultaneous Assessment & 0.5217               & 0.3907               & 0.5507               & 0.4029               & 0.4783               & 0.3024               & 0.6522               & 0.3548               \\
Summarizer Assessment   & 0.4928               & 0.3538               & 0.4493               & 0.2313               & 0.5217               & 0.3436               & 0.6232               & 0.3888      
\\  

\bottomrule
\end{tabular}}
\caption{
Evaluation of different communication strategies of ChatGPT in C++. 
}
\label{RQ2_C++}
\end{table*}

% \section{Additional \tool Results}
\section{Additional Experimental Setting}
\label{additionalexperimentalsetting}
\subsection{Implementation Details}

For ChatGPT (``gpt-3.5-\textit{turbo-0125}'') and GPT-4 (``gpt-4-\textit{turbo}''), we use the public APIs provided by OpenAI. To mitigate the risk of data leakage and effectively evaluate the methods' ability for SV assessment, we adopt a time-split setting based on the ``commit date'' of vulnerability patches.
Specifically, the vulnerability-related commit after 2023-11-27 of Python, 2023-11-28 of Java, and 2023-12-02 of C++ are designated for testing in this paper.

\subsection{Additional Metrics}
We also use the following two widely used performance metrics for SV assessment:

\textbf{Precision:} It is the ratio of true positives ($\text{TP}$) to the sum of true positives and false positives ($\text{FP}$), calculated following: $\text{Precision} = \frac{\text{TP}}{\text{TP}+\text{FP}}$. 

\textbf{Recall:} It is the ratio of $\text{TP}$ to the sum of $\text{TP}$ and false negatives ($\text{FN}$), calculated following: $\text{Recall} = \frac{\text{TP}}{\text{TP}+\text{FN}}$.

\section{Algorithm of Communication Strategies}
\label{AlgorithmofCommunication}
In this appendix, we formally define the following four different communication strategies, including \textit{preceding one expert} (Refer to Algorithm~\ref{algorithm1}), \textit{previous communication}(Refer to Algorithm~\ref{algorithm2}), \textit{simultaneous assessment}(Refer to Algorithm~\ref{algorithm3}), and \textit{summariser assessment}(Refer to Algorithm~\ref{algorithm4}) for the SV assessment task.

\begin{algorithm}[!tpb]
    \footnotesize
    \caption{Referencing the preceding one expert}
    \label{algorithm1}
    \begin{algorithmic}[1]
        \REQUIRE Agents Number: $N$, Expert Agents: $E_{1}, E_{2},\cdots, E_{N}$, Communication Rounds: $R$, Chat History List $History$, Vulnerability Assessment Tasks $T_{1}, T_{2},\cdots, T_{8}$
        \ENSURE Results for Vulnerability Assessment Task $Answer$
        \STATE Initialize a vulnerability assessment task $T_i$
        \FOR{$r \leftarrow 0$ to $R$}
            \FOR{$n \leftarrow 0$ to $N$}
                \IF{$History \neq \emptyset$}
                    \STATE $h_{role} \leftarrow E_n$
                    \STATE $h_{answer} \leftarrow E_n(T_i, History)$
                    \STATE $History \leftarrow \{h_{role}, h_{answer}\}$
                \ELSE
                    \STATE $h_{role} \leftarrow E_n$
                    \STATE $h_{answer} \leftarrow E_n(T_i)$
                    \STATE $History \leftarrow \{h_{role}, h_{answer}\}$
                \ENDIF
                \STATE $Answer \leftarrow$ Final $h_{answer}$
            \ENDFOR
        \ENDFOR
        \RETURN $Answer$
    \end{algorithmic}
\end{algorithm}

\begin{algorithm}[!tpb]
    \footnotesize
    \caption{Referencing the previous communication}
    \label{algorithm2}
    \begin{algorithmic}[1]
        \REQUIRE Agents Number: $N$, Expert Agents: $E_{1}, E_{2},\cdots, E_{N}$, Communication Rounds: $R$, Chat History List $History$, Vulnerability Assessment Tasks $T_{1}, T_{2},\cdots, T_{8}$
        \ENSURE Results for Vulnerability Assessment Task $Answer$
        \STATE Initialize a vulnerability assessment task $T_i$
        \FOR{$r \leftarrow 0$ to $R$}
            \FOR{$n \leftarrow 0$ to $N$}
                \IF{$History \neq \emptyset$}
                    \STATE $h_{role} \leftarrow E_n$
                    \STATE $h_{answer} \leftarrow E_n(T_i, History)$
                    \STATE $History \leftarrow \{h_{role}, h_{answer}\}$
                \ELSE
                    \STATE $h_{role} \leftarrow E_n$
                    \STATE $h_{answer} \leftarrow E_n(T_i)$
                    \STATE $History \leftarrow History + \{h_{role}, h_{answer}\}$
                \ENDIF
                \STATE $Answer \leftarrow$ Final $h_{answer}$
            \ENDFOR
        \ENDFOR
        \RETURN $Answer$
    \end{algorithmic}
\end{algorithm}
\begin{algorithm}[!tpb]
    \footnotesize
    \caption{Simultaneous Assessment}
    \label{algorithm3}
    \begin{algorithmic}[1]
        \REQUIRE Agents Number: $N$, Expert Agents: $E_{1}, E_{2},\cdots, E_{N}$, Communication Rounds: $R$, Chat History List $History$, Vulnerability Assessment Tasks $T_{1}, T_{2},\cdots, T_{8}$
        \ENSURE Results for Vulnerability Assessment Task $Answer$
        \STATE Initialize a vulnerability assessment task $T_i$
        \FOR{$r \leftarrow 0$ to $R$}
            \STATE Initialize current round chat history $History_{c}$
            \FOR{$n \leftarrow 0$ to $N$}
                \IF{$History \neq \emptyset$}
                    \STATE $h_{role} \leftarrow E_n$
                    \STATE $h_{answer} \leftarrow E_n(T_i, History)$
                    \STATE $History_{c} \leftarrow \{h_{role}, h_{answer}\}$
                \ELSE
                    \STATE $h_{role} \leftarrow E_n$
                    \STATE $h_{answer} \leftarrow E_n(T_i)$
                    \STATE $History_{c} \leftarrow \{h_{role}, h_{answer}\}$
                \ENDIF
            \ENDFOR
            \STATE $History \leftarrow History + History_{c}$
            \STATE $Answer \leftarrow$ Final $h_{answer}$
        \ENDFOR
        \RETURN $Answer$
    \end{algorithmic}
\end{algorithm}
\begin{algorithm}[!tpb]
    \footnotesize
    \caption{Summarizer Assessment}
    \label{algorithm4}
    \begin{algorithmic}[1]
        \REQUIRE Agents Number: $N$, Expert Agents: $E_{1}, E_{2},\cdots, E_{N-1}$, Summarizer Agent $S$, Communication Rounds: $R$, Chat History List $History$, Vulnerability Assessment Tasks $T_{1}, T_{2},\cdots, T_{8}$
        \ENSURE Results for Vulnerability Assessment Task $Answer$
        \STATE Initialize a vulnerability assessment task $T_i$
        \FOR{$r \leftarrow 0$ to $R$}
            \STATE Initialize current round chat history $History_{c}$
            \FOR{$n \leftarrow 0$ to $N$}
                \IF{$n \neq N$}
                    \STATE $h_{role} \leftarrow E_n$
                    \STATE $h_{answer} \leftarrow E_n(T_i, History)$
                    \STATE $History_{c} \leftarrow \{h_{role}, h_{answer}\}$
                \ELSE
                    \STATE $s_{role} \leftarrow S$
                    \STATE $s_{answer} \leftarrow S(T_i, History + History_{c})$
                    \STATE $History_{c} \leftarrow \{s_{role}, s_{answer}\}$
                \ENDIF
            \ENDFOR
            \STATE $History \leftarrow History + History_{c}$
            \STATE $Answer \leftarrow$ Final $s_{answer}$
        \ENDFOR
        \RETURN $Answer$
    \end{algorithmic}
\end{algorithm}

\section{Task-related Prompt}
\label{taskrelatedprompt}
In this appendix, we present the task-related prompt by CVSS v3.1 and
design several descriptions as follows.

\textbf{Attack Vector}: \textit{You are a [Language] expert for Attack Vector. This metric reflects the context in which vulnerability exploitation is possible. \ This metric value (and consequently the Base Score) will be larger the more remote (logically, and physically) an attacker can be to exploit the vulnerable component. Network (N): The vulnerable component is bound to the network stack and the set of possible attackers extends beyond the other options listed below, up to and including the entire Internet. Local (L): The vulnerable component is not bound to the network stack and the attacker’s path is via read/write/execute capabilities.}

\textbf{Attack Complexity}: \textit{You are a [Language] expert for Attack Complexity. This metric describes the conditions beyond the attacker’s control that must exist in order to exploit the vulnerability. If a specific configuration is required for an attack to succeed, the Base metrics should be scored assuming the vulnerable component is in that configuration. The Base Score is greatest for the least complex attacks.
Low (L): Specialized access conditions or extenuating circumstances do not exist. An attacker can expect repeatable success when attacking the vulnerable component.
High (H): A successful attack depends on conditions beyond the attacker's control. That is, a successful attack cannot be accomplished at will, but requires the attacker to invest in some measurable amount of effort in preparation or execution against the vulnerable component before a successful attack can be expected.}

\textbf{Privileges Required}: \textit{You are a [Language] expert for Privileges Required. This metric describes the level of privileges an attacker must possess before successfully exploiting the vulnerability. The Base Score is greatest if no privileges are required.
None (N): The attacker is unauthorized prior to attack, and therefore does not require any access to settings or files of the vulnerable system to carry out an attack.
Low (L): The attacker requires privileges that provide basic user capabilities that could normally affect only settings and files owned by a user.
High (H): The attacker requires privileges that provide significant (e.g., administrative) control over the vulnerable component allowing access to component-wide settings and files.}

\textbf{User Interaction}: \textit{You are a [Language] expert for User Interaction. This metric captures the requirement for a human user, other than the attacker, to participate in the successful compromise of the vulnerable component. This metric determines whether the vulnerability can be exploited solely at the will of the attacker, or whether a separate user (or user-initiated process) must participate in some manner. The Base Score is greatest when no user interaction is required.
None (N): The vulnerable system can be exploited without interaction from any user.
Required (R): Successful exploitation of this vulnerability requires a user to take some action before the vulnerability can be exploited.}

\textbf{Scope}: \textit{You are a [Language] expert for Scope. The Scope metric captures whether a vulnerability in one vulnerable component impacts resources in components beyond its security scope. The Base Score is greatest when a scope change occurs.
Unchanged (U): An exploited vulnerability can only affect resources managed by the same security authority.
Changed (C): An exploited vulnerability can affect resources beyond the security scope managed by the security authority of the vulnerable component.}

\textbf{Confidentiality}: \textit{You are a [Language] expert for Confidentiality. This metric measures the impact to the confidentiality of the information resources managed by a software component due to a successfully exploited vulnerability. The impact can vary from none to complete disclosure of all restricted information to the attacker.
High (H): There is a total loss of confidentiality, resulting in all resources within the impacted component being divulged to the attacker. Alternatively, access to only some restricted information is obtained, but the disclosed information presents a direct, serious impact.
Low (L): There is some loss of confidentiality. Access to some restricted information is obtained, but the attacker does not have control over what information is obtained, or the amount or kind of loss is limited.
None (N): There is no loss of confidentiality within the impacted component.}

\textbf{Integrity}: \textit{You are a [Language] expert for Integrity. This metric measures the impact to the integrity of a successfully exploited vulnerability. Integrity refers to the trustworthiness and veracity of information. The Base Score is greatest when the consequence to the impacted component is highest.
High (H): There is a total loss of integrity, or a complete loss of protection. For example, the attacker is able to modify any/all files protected by the impacted component.
Low (L): Modification of data is possible, but the attacker does not have control over the consequence of a modification, or the amount of modification is limited.
None (N): There is no loss of integrity within the impacted component.}

\textbf{Availability}: \textit{You are a [Language] expert for Availability. This metric measures the impact to the availability of the impacted component resulting from a successfully exploited vulnerability. The Base Score is greatest when the consequence to the impacted component is highest.
High (H): There is a total loss of availability, resulting in the attacker being able to fully deny access to resources in the impacted component; this loss is either sustained (while the attacker continues to deliver the attack) or persistent (the condition persists even after the attack has completed).
Low (L): Performance is reduced or there are interruptions in resource availability. Even if repeated exploitation of the vulnerability is possible, the attacker does not have the ability to completely deny service to legitimate users.
None (N): There is no impact to availability within the impacted component.}
