# Supplementary material for: EvalSVA: Multi-Agent Evaluators for Next-Gen Software Vulnerability Assessment
Source: arXiv:2501.14737 source file (2024-12-11)
Supplement: Supplementary file 2 [file RQ2_C++_Appendix.tex]

\begin{table*}[t]
\centering
\setlength{\tabcolsep}{3.5mm}

\resizebox{\textwidth}{!}{
\begin{tabular}{lcccccccc}
\toprule
\textit{\textbf{Exploitability Metrics}}  & \multicolumn{2}{c}{\textbf{AV}}       & \multicolumn{2}{c}{\textbf{AC}}       & \multicolumn{2}{c}{\textbf{PR}}       & \multicolumn{2}{c}{\textbf{UI}}       \\

\textit{\textbf{Communication Strategy}} & \textbf{Acc} & \textbf{F1} & \textbf{Acc} & \textbf{F1} & \textbf{Acc} & \textbf{F1} & \textbf{Acc} & \textbf{F1} \\
\toprule
Single Agent            & 0.3333               & 0.3088               & 0.2754               & 0.1873               & 0.1449               & 0.0921               & 0.5072               & 0.4569               \\
Previous Communication  & 0.2319               & 0.2214               & 0.3333               & 0.1950               & 0.6087               & 0.2523               & 0.5507               & 0.5473               \\
Preceding One Expert    & 0.4203               & 0.3611               & 0.4203               & 0.2372               & 0.5942               & 0.2485               & 0.5652               & 0.5629               \\
Simultaneous Assessment & 0.1884               & 0.1869               & 0.3913               & 0.2129               & 0.6812               & 0.2701               & 0.5072               & 0.5063               \\
Summarizer Assessment   & 0.2899               & 0.2746               & 0.4928               & 0.2686               & 0.6957               & 0.3058               & 0.5072               & 0.5071               \\
\bottomrule
\specialrule{0em}{2pt}{2pt}
\toprule
\textit{\textbf{Scope and Impact Metrics}}  & \multicolumn{2}{c}{\textbf{S}}        & \multicolumn{2}{c}{\textbf{C}}        & \multicolumn{2}{c}{\textbf{I}}        & \multicolumn{2}{c}{\textbf{A}}        \\

\textit{\textbf{Communication Strategy}} & \textbf{Acc} & \textbf{F1} & \textbf{Acc} & \textbf{F1} & \textbf{Acc} & \textbf{F1} & \textbf{Acc} & \textbf{F1}         \\
\toprule
Single Agent            & 0.1449               & 0.1384               & 0.4638               & 0.2622               & 0.4928               & 0.3192               & 0.5072               & 0.2509               \\
Previous Communication  & 0.4203               & 0.3155               & 0.4928               & 0.3074               & 0.4348               & 0.2259               & 0.6812               & 0.4059               \\
Preceding One Expert    & 0.4928               & 0.3538               & 0.5072               & 0.3616               & 0.4203               & 0.2920               & 0.5942               & 0.3459               \\
Simultaneous Assessment & 0.5217               & 0.3907               & 0.5507               & 0.4029               & 0.4783               & 0.3024               & 0.6522               & 0.3548               \\
Summarizer Assessment   & 0.4928               & 0.3538               & 0.4493               & 0.2313               & 0.5217               & 0.3436               & 0.6232               & 0.3888      
\\  

\bottomrule
\end{tabular}}
\caption{
Evaluation of different communication strategies of ChatGPT in C++. 
}
\label{RQ2_C++}
\end{table*}
