# Supplementary material for: EvalSVA: Multi-Agent Evaluators for Next-Gen Software Vulnerability Assessment
Source: arXiv:2501.14737 source file (2024-12-11)
Supplement: Supplementary file 3 [file RQ2_Java_Appendix.tex]

\begin{table*}[t]
\centering
\setlength{\tabcolsep}{3.5mm}

\resizebox{\textwidth}{!}{
\begin{tabular}{lcccccccc}
\toprule
\textit{\textbf{Exploitability Metrics}}  & \multicolumn{2}{c}{\textbf{AV}}       & \multicolumn{2}{c}{\textbf{AC}}       & \multicolumn{2}{c}{\textbf{PR}}       & \multicolumn{2}{c}{\textbf{UI}}       \\

\textit{\textbf{Communication Strategy}} & \textbf{Acc} & \textbf{F1} & \textbf{Acc} & \textbf{F1} & \textbf{Acc} & \textbf{F1} & \textbf{Acc} & \textbf{F1} \\
\toprule
Single Agent            & 0.4778 & 0.4075 & 0.4000 & 0.3132 & 0.2889 & 0.2425 & 0.3667 & 0.3532 \\
Previous Communication  & 0.3222 & 0.3078 & 0.4444 & 0.2167 & 0.5778 & 0.3603 & 0.5000 & 0.4994 \\
Preceding One Expert    & 0.3111 & 0.3056 & 0.3556 & 0.1943 & 0.5556 & 0.3492 & 0.4667 & 0.4643 \\
Simultaneous Assessment & 0.4444 & 0.3939 & 0.4111 & 0.2158 & 0.5778 & 0.3613 & 0.4222 & 0.4219 \\
Summarizer Assessment   & 0.4889 & 0.4564 & 0.3222 & 0.1728 & 0.5333 & 0.3387 & 0.4000 & 0.4000 \\
\bottomrule
\specialrule{0em}{2pt}{2pt}
\toprule
\textit{\textbf{Scope and Impact Metrics}}  & \multicolumn{2}{c}{\textbf{S}}        & \multicolumn{2}{c}{\textbf{C}}        & \multicolumn{2}{c}{\textbf{I}}        & \multicolumn{2}{c}{\textbf{A}}        \\

\textit{\textbf{Communication Strategy}} & \textbf{Acc} & \textbf{F1} & \textbf{Acc} & \textbf{F1} & \textbf{Acc} & \textbf{F1} & \textbf{Acc} & \textbf{F1}         \\
\toprule
Single Agent            & 0.1444 & 0.1392 & 0.5111 & 0.2591 & 0.4556 & 0.2406 & 0.4556 & 0.2427 \\
Previous Communication  & 0.3333 & 0.3168 & 0.5333 & 0.3457 & 0.5000 & 0.2496 & 0.4556 & 0.2169 \\
Preceding One Expert    & 0.3778 & 0.3623 & 0.5333 & 0.3572 & 0.4889 & 0.2729 & 0.4222 & 0.2189 \\
Simultaneous Assessment & 0.3444 & 0.3202 & 0.5000 & 0.2582 & 0.5111 & 0.2495 & 0.4667 & 0.2390 \\
Summarizer Assessment   & 0.4000 & 0.3619 & 0.5333 & 0.2819 & 0.4889 & 0.2731 & 0.4667 & 0.2317       
\\  

\bottomrule
\end{tabular}}
\caption{
Evaluation of different communication strategies of ChatGPT in Java. 
}
\label{RQ2_Java}
\end{table*}
